# Supplementary material for: Near-threshold photoelectron holography beyond the strong-field approximation
Source: arXiv:1703.04123 ancillary file (2017-03-15)
Supplement: Supplementary file 1 [file Supplemental_material.pdf]

# Supplemental material for
# Near-threshold photoelectron holography beyond the strong-field approximation

XuanYang Lai[1], ShaoGang Yu[1,2], YiYi Huang[1,2], LinQiang Hua[1], Cheng Gong[1], Wei Quan[1], C. Figueira de Morisson Faria[3], and XiaoJun Liu[1]

[1] *State Key Laboratory of Magnetic Resonance and Atomic and Molecular Physics and Center for Cold Atom Physics, Wuhan Institute of Physics and Mathematics, Chinese Academy of Sciences, Wuhan 430071, China*

[2] *School of Physics, University of Chinese Academy of Sciences, Beijing 100080, China*

[3] *Department of Physics and Astronomy, University College London, Gower Street, London WC1E 6BT, United Kingdom*

We provide additional information on how the photoelectron angular distributions (PADs) are calculated using the Coulomb Quantum-Orbit Strong-Field Approximation (CQSFA), how this approach differs from existing Coulomb-corrected strong-field theories, the influence of the target and laser parameters on the PADs and on possible reasons for the discrepancy between our results and those obtained with the numerical solution of the time-dependent Schrödinger equation (TDSE).

## I. TRANSITION AMPLITUDE IN THE COULOMB QUANTUM-ORBIT STRONG-FIELD APPROXIMATION

Below we briefly outline how the ATI transition amplitude is computed in the Coulomb quantum-orbit strong-field approximation (CQSFA). For more details, please see Ref. [1]. The Coulomb-corrected transition amplitude for any given final momentum $\mathbf{p}_f$ is written as

$$M(\mathbf{p}_f) \propto -i \lim_{t\to\infty} \sum_s \left\{ \det \left[ \frac{\partial \mathbf{p}_s(t)}{\partial \mathbf{r}_s(t_{0,s})} \right] \right\}^{-1/2} e^{iS(\tilde{\mathbf{p}}_s,\mathbf{r}_s,t_{0,s},t))} \times \mathcal{C}(t_{0,s}) \left\langle \mathbf{p}_s(t_{0,s}) + \mathbf{A}(t_{0,s}) \left| \hat{H}_I(t_{0,s}) \right| \psi_0 \right\rangle , \quad (1)$$

where the term $\mathcal{C}(t_0) = \sqrt{2\pi i/(\partial^2 S/\partial t_0^2)}$ is the prefactor, $\partial \mathbf{p}(t)/\partial \mathbf{r}(t_0)$ is related to the stability of the trajectory, and the index $s$ denotes the different quantum orbits from three saddle-point equations,

$$[\mathbf{p}_0 + \mathbf{A}(t_0)]^2/2 + I_p = 0, \quad (2)$$

$$\dot{\mathbf{p}}(\tau) = -\nabla_{\mathbf{r}} V[\mathbf{r}(\tau)], \quad (3)$$

and

$$\dot{\mathbf{r}}(\tau) = \mathbf{p}(\tau) + \mathbf{A}(\tau), \quad (4)$$

which are solved using an iteration scheme for any given final momentum with the assumption that the electron is ionized by tunneling from $t_0$ to $t_0^R = \mathrm{Re}[t_0]$. Once the electron is in the continuum, all variables are taken to be real. The tunnel exit is chosen according to Refs. [2, 3].

First of all, we solve the CQSFA trajectories from the Coulomb-corrected saddle-point solutions (2)-(4). There are four types of trajectories for each photoelectron with any given final momentum [1]. Here, we assume that the laser polarization is along the $z$ axis and the final momentum along the laser polarization $p_{f,z} > 0$. For trajectories of type I, the tunneling exit $z_0 > 0$, and the electron moves directly towards the detector without returning to its parent ion. For the type II and III trajectories, the tunneling exit $z_0 < 0$, meaning that the initial motion carries the electron away

from the detector before it turns around and finally arrives with the stipulated momentum $\mathbf{p}_f$. A closer inspection shows that they are similar to Kepler hyperbolae to which a drift motion caused by the field is superimposed [4, 5]. Trajectory types I and II are similar to the so-called "short" and "long" trajectories in the SFA theory. Trajectory type III is not found in the SFA and can be observed after the Coulomb potential is considered. This is consistent with Ref. [5], where this classification was first introduced. In more strict terms, however, our previous results show that orbit II is twofold degenerate in the SFA, and that the presence of the Coulomb potential lifts this degeneracy [1].

Additionally, our computations uncover an additional trajectory type, denoted as IV. For this type of orbit, although the tunnel exit points towards the detector, the electron is driven back to the core by the laser field, then goes around the core, and finally moves towards to the detector. With increasing photoelectron final momentum, the shortest distance between the electron and the core decreases [1]. This distance can be smaller than the tunnel exit. In this case, this type of trajectory corresponds to a rescattering event. It is noteworthy that our numerical simulations show that only type I-III trajectories are needed for obtaining converged photoelectron spectra in the low-energy region [1]. Illustrations of these types of trajectories are provided in our previous publication [1].

Next, we calculate the action of each trajectory

$$S(\tilde{\mathbf{p}}, \mathbf{r}, t_0, t) = I_p t_0 - \int_{t_0}^{t} d\tau [\dot{\mathbf{p}} \cdot \mathbf{r}(\tau) + H(\mathbf{r}(\tau), \mathbf{p}(\tau), \tau)], \tag{5}$$

where $I_p$ is the ionization potential and $H(\mathbf{r}(\tau), \mathbf{p}(\tau), \tau) = \frac{1}{2}\left[\mathbf{p}(\tau) + \mathbf{A}(\tau)\right]^2 - \frac{1}{\sqrt{\mathbf{r}(\tau)\cdot\mathbf{r}(\tau)}}$ (for details about this derivation see our previous publication [1]). In practice, we assume that the momentum of the electron is fixed during the tunneling ionization. In this case, the second term on the right-hand side of Eq. (5) is split into a part inside the barrier,

$$\tilde{S}^{\mathrm{in}}(\tilde{\mathbf{p}}, \mathbf{r}, t_0, t) = -\int_{t_0}^{t_0^R} H(\mathbf{r}, \mathbf{p}, \tau) d\tau \tag{6}$$

with the tunneling trajectory $\mathbf{r}_s(t) = \int_{t_s}^{t} [\mathbf{p}_s(\tau) + \mathbf{A}(\tau)] d\tau$ [2] and a part outside the barrier,

$$\tilde{S}^{\mathrm{out}}(\tilde{\mathbf{p}}, \mathbf{r}, t_0, t) = \int_{t_0^R}^{t} d\tau [-\dot{\mathbf{p}}(\tau) \cdot \mathbf{r}(\tau) - H(\mathbf{r}, \mathbf{p}, \tau)], \tag{7}$$

with the ionization trajectory determined by Eq. (4).

Thereafter, we calculate the stability of the trajectories numerically. In practice, instead of using $\partial \mathbf{p}_s(t)/\partial \mathbf{r}_s(t_s)$ in Eq. (1) we employ $\partial \mathbf{p}_s(t)/\partial \mathbf{p}_s(t_s)$. The latter stability factor is of easier implementation, and can be obtained using a Legendre transformation in the transition amplitude (1). Upon this transformation, the action will remain the same as long as the electron starts from the origin. For details on Legendre transformations see, e.g., [6]. The normalization constants in the above-stated equations are such that, in the limit of vanishing binding potential, the SFA transition amplitude is recovered.

Finally, we calculate the form factor, $\langle \mathbf{p}(t_0) + \mathbf{A}(t_0) \, | \hat{H}_I(t_0) | \, \psi_0 \rangle$, with $\hat{H}_I(t_0) = -\hat{\mathbf{r}} \cdot \mathbf{E}(t_0)$. In our work, the initial state is taken as the ground state of Hydrogen atom, $\psi_0(\mathbf{r}) = e^{-r}/\sqrt{\pi}$. In this case, the tunnel matrix element in Eq. (1) becomes related to the atomic dipole moment and can be simplified as $\langle \mathbf{p}(t_0) + \mathbf{A}(t_0) \, | - \mathbf{r} \cdot \mathbf{E}(t_0) | \, \psi_0 \rangle \sim E(t_0) \tilde{p}_{0z}$ in a linearly polarized laser field, where $\tilde{\mathbf{p}}_0 = \mathbf{p}(t_0) + \mathbf{A}(t_0)$ [7].

## II. ADVANTAGES AND LIMITATIONS OF THE CQSFA THEORY

The CQSFA is very propitious for computing two-dimensional PADs and assessing quantum-interference effects such as the structure discussed in this work, for the reasons stated below:

1. It provides a transparent picture in terms of electron orbits leaving its parent ion and reaching the detector, whose contributions can be switched on and off at will. This is an advantage over purely numerical methods such as the TDSE, which contains no physical approximations, but for which different features are more difficult to disentangle.

2. It accounts for tunneling and quantum interference effects. This means that it may be used directly to construct a fan-shaped structure and accounts for phase differences between different types of trajectories, while purely classical approaches, such as the Classical Trajectory Monte Carlo Method (CTMC) require indirect arguments and means in order to infer the underlying physics behind it [4].

3. In contrast to methods such as the Coulomb Volkov approximation [8], it incorporates the Coulomb potential in the electron propagation and not only in its final state. Hence, it can provide information about how it influences the phases of different types of electron trajectories.

4. In principle, other approaches such as the Eikonal Volkov Approximation (EVA) [9] and the Coulomb-corrected SFA (CCSFA) [5] also account for 1.–3. In practice, however, the EVA requires small scattering angles, which may render its implementation difficult for computing PADs. Furthermore, the CCSFA requires a large number of orbits as it currently solves the direct and not the inverse problem, which makes the extraction of phase information from PADs more cumbersome [5]. In contrast, the CQSFA does not require any restriction upon the scattering angle and requires only a few orbits for obtaining converged PADs.

Our method, however, does not exhibit a quantitative agreement with the TDSE. For example, Fig. 1 shows that the TDSE yield decays much faster with increasing scattering angle than for the CQSFA. This may be related to the following issues.

In the TDSE, the initial electronic wavepacket has an initial momentum and position spread, while all CQSFA orbits are located at the tunnel exit. This may reduce the subsequent wavepacket spread and lead to a slight over-enhancement of the contributions for non-vanishing scattering angles. Indeed, there is significant evidence, in the context of high-order harmonic generation (HHG), that the initial spread of the electronic wave packet is necessary for

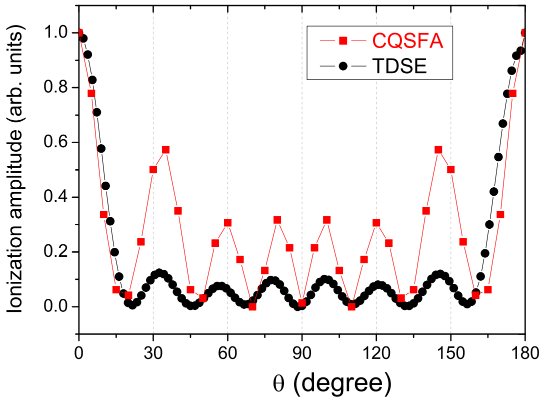


FIG. 1: (Color online) Angular distributions of the photoelectron in the first ATI ring with the momentum around 0.2 a.u. for the hydrogen atom ($I_p = 0.5$ a.u.) in a linearly polarized laser field of intensity $I = 2 \times 10^{14}$ W/cm$^2$ and wavelength $\lambda = 800$ nm. The square curve in red and the circle curve in black refer to the CQSFA and TDSE solutions, respectively. The amplitude has been normalized to the maximum value.

a good quantitative agreement with the TDSE [10–13]. Neglect of this spread leads to overall changes in the harmonic intensities [13] and an over-enhancement of the contributions of the long orbit in the HHG spectra [10, 11, 13]. This initial spread seems to be very important for strong-field ionization as well, as recent phase-space studies revealed that orbit-based methods that incorporate this spread exhibit a nearly quantitative agreement with the TDSE, even if tunnel ionization is not properly accounted for [14].

## III. TARGET DEPENDENCE OF THE FAN-SHAPED STRUCTURE

In our work, we have shown that the appearance of the fan-shaped structure depends on the target's potential, which is long-range. For the short range potential, e.g., the ionization of the negative ion, the influence of the ionic Coulomb potential is negligible and hence, no fan shaped structure can be observed [see Fig. 1(b) in the main body of the paper]. Apart from that, we have assumed that the electron is freed from the ground state of hydrogen atom with spherical symmetry, $\psi_0(\mathbf{r}) = e^{-r}/\sqrt{\pi}$. Indeed, we find that the symmetry of the initial electronic state also significantly influences the fan-shaped structure. If we employ an antisymmetric initial state, e.g., $\psi_0(\mathbf{r}) \sim e^{-r}\cos\theta$, and keep the same binding energy (0.5 a.u.), the tunnel matrix element in Eq. (1) becomes $\langle \mathbf{p}(t) + \mathbf{A}(t) \mid -\mathbf{r}\cdot\mathbf{E}(t) \mid \psi_0\rangle \sim E(t)\tilde{p}_{0z}^2$. Fig. 2 shows the CQSFA simulations of the two-dimensional PADs near the ionization threshold in a linearly polarized laser field for the two kinds of the initial states. As one can see, for the initial state with spherical symmetry, there are eight peaks in the first ATI ring, as mentioned in the main body of the paper, while for the state with antisymmetry, only 7 peaks can be observed in the first ATI ring. The reason for the divergence is that for the state with antisymmetry, there is an additional phase difference of $\pi$ between the direct trajectory and the forward-rescattering trajectory during the tunneling ionization [15]. This results in the different interference patterns: The peaks in the first ATI ring for the initial state with spherical symmetry are suppressed for the state with antisymmetry, while the ionization suppression in the first ATI ring for the state with spherical symmetry becomes enhanced for the state with antisymmetry. Therefore, our simulation shows that the fan-shaped pattern is closely related to the target structures, which can be used to extract the information of the target's structure by analyzing the fan-shaped structure in the two-dimensional PADs. It is worthy to note that our

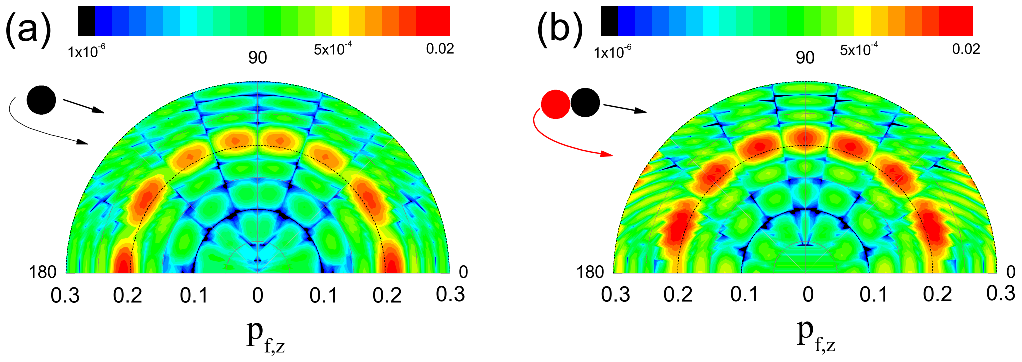


FIG. 2: (Color online) CQSFA simulations of the two-dimensional PADs near the ionization threshold in a linearly polarized laser field. (a) for the initial state of $\psi_0(\mathbf{r}) = e^{-r}/\sqrt{\pi}$, and (b) for the initial state of $\psi_0(\mathbf{r}) \sim e^{-r}\cos\theta$. The momentum component along the laser polarization direction is given by $p_{f,z}$. The schematic diagram on the left side denotes the orbital symmetry of the initial state and the interference trajectories. The parameters of the laser field are the same as that in the main body of the paper.

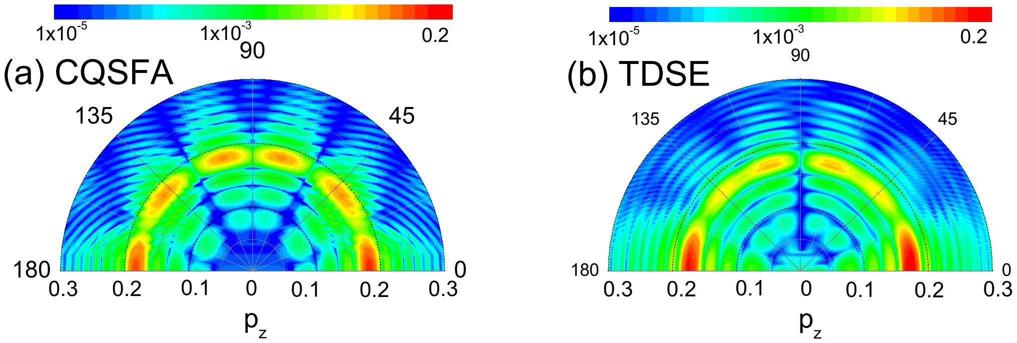


FIG. 3: (Color online) Same as Figs. 1(a) and 1(c) in the main body of the paper, but with the different laser intensity of $I = 5{\times}10^{13}$ W/cm$^2$.

results are different from the previous publications, in which the influence of the symmetry of the initial state on the fan-shaped structure is neglected. For example, Chen et al [16] proposed an empirical rule for the dominant orbital angular momentum in the fan-like pattern, which was only determined by the number of photons absorbed. Arbó et al [4] studies the near-threshold radial pattern in terms of a CTMC method with tunneling and found that the dominant angular momentum in the fan-like patterns is virtually independent of the atomic species.

## IV. LASER-PARAMETER DEPENDENCE OF THE FAN-SHAPED STRUCTURE IN THE CQSFA SIMULATIONS

In the main body of the paper, we have shown the fan-shaped structure in the laser field of intensity of $I = 2{\times}10^{14}$ W/cm$^2$ and wavelength $\lambda = 800$ nm (Keldysh parameter $\gamma = \sqrt{I_p/2U_p} = 0.75$ [17]). However, there are plenty of examples in the literature, both theoretical and experimental, for which this structure is reproduced in different regimes, such as the multiphoton ionization regime or the deeply tunneling ionization regime (e.g., low-frequency, mid-IR regime). In these regimes, the number of peaks of the fan-shaped structure is changed, but not the pattern [4, 16]. Indeed, we have also simulated the fan-shaped structure with CQSFA theory using different laser parameters, for example, $I = 5{\times}10^{13}$ W/cm$^2$ ($\gamma = 1.5$; see Fig. 3). In the figure, there are only six peaks left in the first above-threshold ionization ring at the momentum $p_f \sim 1.8$ a.u, but the fan-shaped structure is still present. Moreover, the overall interference pattern in CQSFA qualitatively exhibits a good agreement with the TDSE simulations in Fig. 3(b), including the correct number of the peaks.

[1] X. Y. Lai, C. Poli, H. Schomerus, and C. Figueira de Morisson Faria, Phys. Rev. A **92**, 043407 (2015).
[2] S.V. Popruzhenko and D. Bauer, J. Mod. Opt. **55**, 2573 (2008).
[3] S. V. Popruzhenko, J. Phys. B **47**, 204001 (2014).
[4] D. G. Arbó *et al.*, Phys. Rev. Lett. **96**, 143003 (2006); D. G. Arbó *et al.*, Phys. Rev. A **78**, 013406 (2008).
[5] T. M. Yan, S. V. Popruzhenko, M. J. J. Vrakking, and D. Bauer, Phys. Rev. Lett. **105**, 253002 (2010).
[6] H. Goldstein, C. P. Poole and J. L. Safko, *Classical Mechanics* (Addison Wesley, 2002)
[7] D. B. Milošević, G. G. Paulus, D. Bauer and W. Becker, J. Phys. B **39**, R203 (2006).
[8] D. G. Arbó *et al.*, Phys. Rev. A **77**, 013401 (2008).

[9] O. Smirnova, M. Spanner, and M. Ivanov, Phys. Rev. A **77**, 033407 (2008).

[10] M. B. Gaarde and K. J. Schafer, Phys. Rev. A **65**, 031406(R) (2002).

[11] J. A. Pérez-Hernández, J. Ramos, L. Roso, and L. Plaja, Laser Phys. **20**, 1044 (2010).

[12] J. Wu, B. B. Augstein and C. Figueira de Morisson Faria, Phys. Rev. A **88**, 023415 (2013).

[13] J. Wu, B. B. Augstein and C. Figueira de Morisson Faria, Phys. Rev. A **88**, 063416 (2013).

[14] C. Zagoya, J. Wu, M. Ronto, D. V. Shalashilin, C. Figueira de Morisson Faria, New J. Phys. **16**, 103040 (2014).

[15] D. B. Milošević *et al.*, Phys. Rev. A **76**, 053410 (2007).

[16] Z. Chen *et al.*, Phys. Rev. A **74**, 053405 (2006).

[17] L. V. Keldysh, Zh. Eksp. Teor. Fiz.**47**, 1945 (1964) [Sov. Phys. JETP20, 1307 (1965)].
